# Supplementary material for: A path forward: Improving Internet routing security by enabling zones of trust
Source: arXiv:2312.03305 source file (2023-12-06)
Supplement: Supplementary file 1 [file appendix-hurricane.tex]

\section{Understanding the residual risk: U.S. case study}
\label{sec:usg-fcc}

By design, our proposed approach does not seek to protect every part
of the Internet.
Our proposal provides protection from invalid origin and invalid path
hijacks to ASes that are in the VIPzone, and to customers that are directly
connected to transit providers in the VIPzone.
The VIPzone leaves ASes that are not in those classes no better
\kc{we mean worse?} off than
today. We try to estimate what fraction of ASes are protected,
and the character (size, routing footprint) of those that are not protected.

For this analysis, we consider the actual Internet AS-level
topology, including provider-customer and peering relationships.
Relevant aspects of this topology, such as the AS path length
from the periphery to core (Tier 1) ISPs, varies by region and
over time. Deployment of our scheme would likely induce changes in
how AS operators configure their (transit and peering) interconnections.

Motivated tby the FCC's recent Notice of Inquiry \cite{fcc-noi-2022},
we use the U.S. as a case study to explore a hypothetical
deployment scenario and its residual risks of hijacks.  Assume
that the MANRS program expanded such that any U.S. network
operator (AS) with more than 100 customer ASes (aggregating
across all the ASes that belong to that organization) complied
with the proposed enhanced practices and became part of the VIPzone.
What would protection of the U.S. region of the Internet look like in
this case?

We use data from CAIDA's AS Rank service (1 December 2022)
to estimate the number
and types of ASes receiving protection from this scenario.  Note that
these numbers rely on a current publically observable state of the
Internet's AS topology, which changes as ISPs change their
interconnection patterns.  They are an approximation to frame the discussion.

\subsection{ASes with only transit interconnections}

\begin{figure*}
\centering \includegraphics[width=.8\textwidth,height=.40\textwidth]{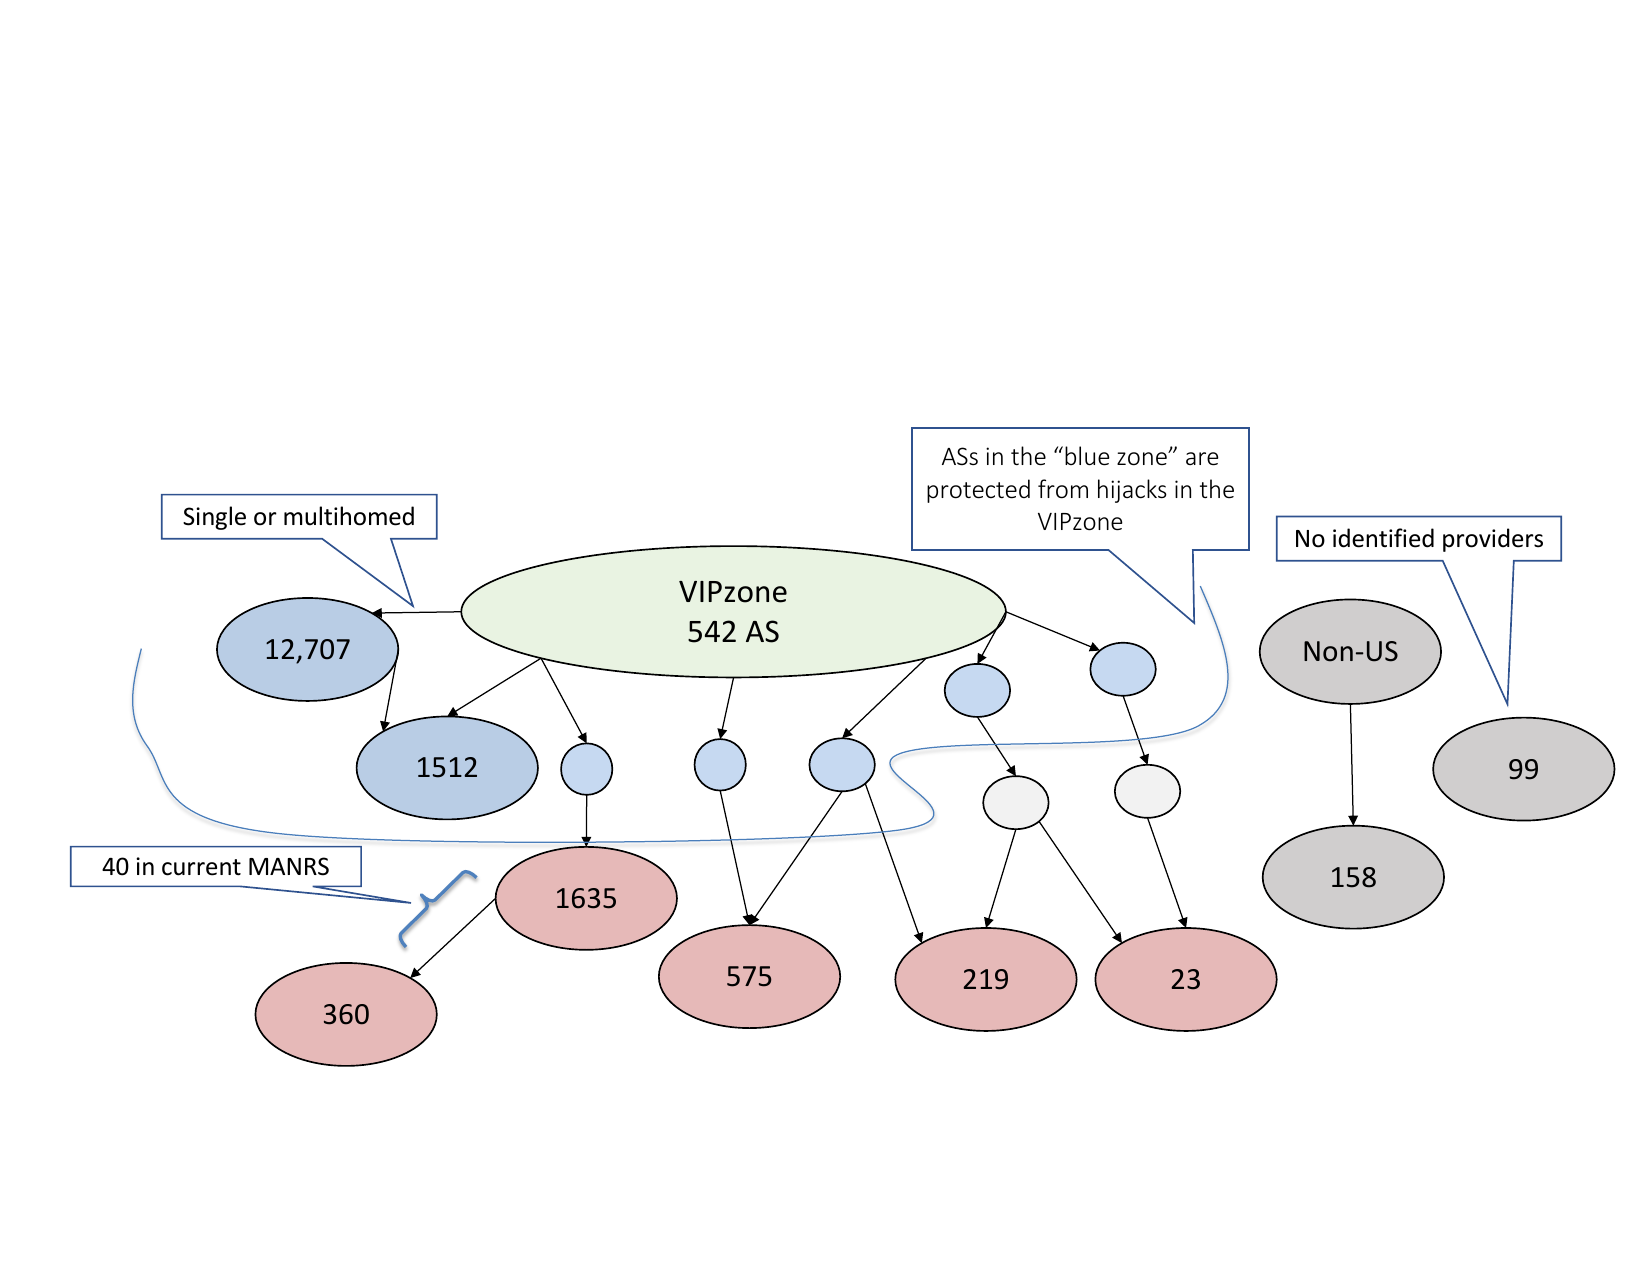}
\caption{\em  The shape of provider-customer connections in the U.S. region of the Internet if all organizations with more than 100 AS customers were in the VIPzone.}
\label{fig:topo}
\vskip -5mm
\end{figure*}

Stipulating that all ASes with greater than 100 customer ASes
are participating in VIPzone practices,
Figure~\ref{fig:topo} depicts the distribution of ASes with different
levels of protection.  An estimated 542 U.S. ASes would be in the VIPzone,
and another 14,219 customer ASes (colored blue) would also benefit from
protection due to their direct transit connection to a provider in the
VIPzone.

These 14,219 ASes include those with the following
interconnection arrangements:

\begin{enumerate}
\item Customers with {\bf only transit provider(s) in the zone:} 12,797.

\item Customers that get transit service {\bf both
from provider(s) in the VIPzone and from provider(s) directly connected to
the zone}: 1,512.

These ASes are protected, but ASes in the VIPzone will always prefer the prefixes of that customer that are
directly announced to the VIPzone.

\item {\bf Single-homed (stub) ASes that are two AS hops away from the VIPzone}:
1635.

\item {\bf Single-homed ASes that are more than two AS hops away from the VIPzone}: 360.

\item {\bf Multi-homed ASes that are more than one hop from the zone}: 817. For these ASes, the hijack risk remains.  In our observation period, these ASes tend to be small institutions (a business, school, etc.).  One would have to decide if the actual risk of hijacks of these small targets is a realistic concern.

\item {\bf U.S.-based ASes that get transit from a non-U.S. provider:}  158.
Most of these are foreign subsidiaries of U.S. firms. To understand what protection the VIPzone could secure for these ASes would require proposing a hypothetical scope for the VIPzone outside the U.S., which we do not attempt to do.

\item {\bf ASes with no observable transit provider:} 99.  Inspection of the data suggests that these are specialized content providers, hosting services, etc. that connect to the Internet only through peering connections.  We analyze
peering interconnections next.
 \end{enumerate}

\subsection{ASes with peering interconnections to and around zone}

Figure~\ref{fig:topo} depicts only transit links i.e., between a
customer and transit provider; peering connections are so dense
that we cannot usefully visualize them.

As mentioned in \S\ref{subsec:vipzone-peering},
peering connections have implications for protection against
hijacks. As a case study, we examine the U.S. ISP with over
100 AS-level customers and also with the
largest number of peering connections: Hurricane Electric (HE).
In our data set, HE has 2079 customers with their own ASN, and 7677 peers
globally, of which 699 are in the U.S.  Of these peers, 76 ASes are
in the VIPzone, 536 are directly connected customers of ASes
in the VIPzone, and only 30 are ASes that are more than one
hop from the zone.
When HE gets announcements from its peers not in the zone, HE should
mark them \ver~ or not based on the practices in \S\ref{sec:design:vipzone}.

The complication for an AS in the VIPzone with peers that are not in the
zone is that some ASes in the customer cone of one of their peers may
also have a connection to another provider that is in the VIPzone
(see \S\ref{subsubsec:transit-and-peering} and Figure~\ref{fig:transitpeering}).
HE's rich peering practices yield 2629 ASes it can reach
both through a peer not in the VIPzone (and thus using announcements that are not~\ver) and
through a peer or customer in the VIPzone, using a path that is \ver.  We assume that HE would prefer
to reach these $\approx$2K ASes over a peering connection, but for most
of them (all but 352) HE has multiple routes via peers to those ASes,
one of which is a peering path inside the VIPzone. This outcome arises
from the rich peering relationships used by HE. Only for the remaining
325 ASes would HE have to decide to forego the peering path and prefer the
\ver~option, or undertake to get accurate knowledge about the customers
of that peer, so that it could implement an exception to the preference
rule and prefer the announcement from the peer that is not \ver.

Our proposal generally assumes it is not practical for an AS to have
accurate knowledge of the customers of its customers, or in this case
its peers. However, it may be practical in specific cases.  If HE were
to prefer this route without having information about the customers of
the peer, it would put its own customers at risk of a hijack originating
in that peer.

\kc{something like this should get in main paper (if not the
whole appendix}
Note that if Hurricane and Cogent finally agreed to peer with
each other, Hurricane would get access via the VIPzone
to 220 of the 325 ASes we consider here. Business practices, not any
technical constraints, will define how the VIPzone protections are
available to various customers.  Deployment of the practices would
likely lead to changes in interconnection practices, and thus the Internet topology,
to evolve in response.
